# Supplementary material for: First-principles prediction of superconductivity in MgB$_3$C$_3$
Source: arXiv:2212.14184 source file (2023-04-03)
Supplement: Supplementary file 1 [file SI.pdf]

# Supplemental Materials: First-Principles Prediction of Superconductivity in $MgB_3C_3$

Truong-Tho Pham[1,2] and Duc-Long Nguyen[3,2,*]

[1] *Laboratory of Magnetism and Magnetic Materials, Science and Technology Advanced Institute, Van Lang University, Ho Chi Minh City, Vietnam*

[2] *Faculty of Applied Technology, School of Technology, Van Lang University, Ho Chi Minh City, Vietnam*

[3] *Laboratory of Applied Physics, Science and Technology Advanced Institute, Van Lang University, Ho Chi Minh City, Vietnam*

(Dated: April 3, 2023)

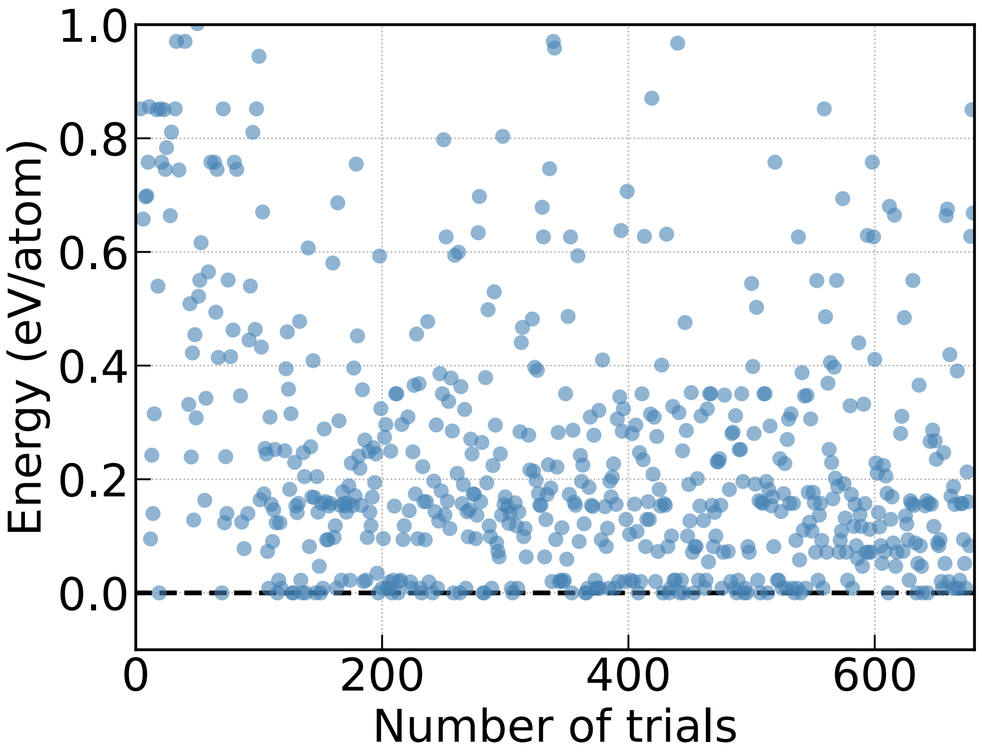


Fig.S 1. Result of crystal structure prediction using evolution algorithm for $MgB_3C_3$. The unit cell of the predicted structure contains one formula unit, which is made up of 7 atoms. The total energy differences of the predicted structure from the most stable structure are plotted as a function of the number of trials within a range of 1 eV/atom.

---

* nguyenduclong@vlu.edu.vn

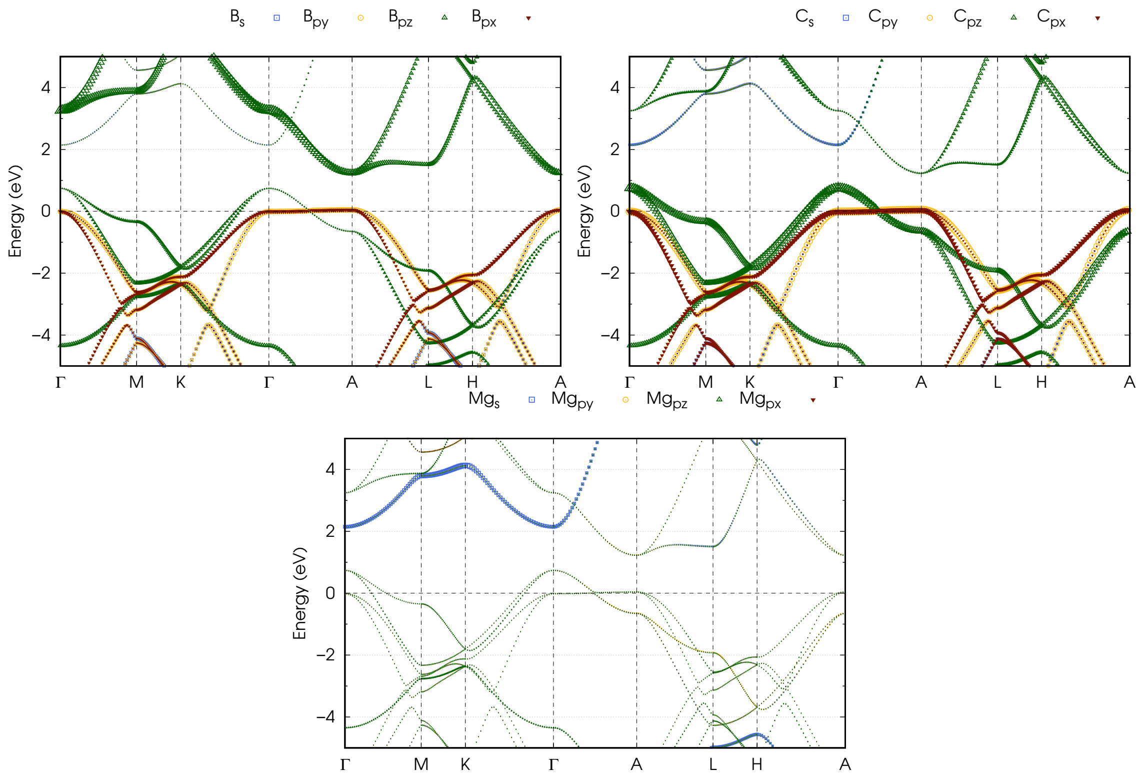


Fig.S 2. The band structure of $MgB_3C_3$, with the orbital contributions of each atom (B, C, and Mg) plotted. The size of the scatter represents the weight of the orbital.
